# Supplementary material for: Bayesian inference for stochastic oscillatory systems using the phase-corrected Linear Noise Approximation
Source: arXiv:2205.05955 source file (2024-07-04)
Supplement: Supplementary file 3 [file BA2205_011_responseLetter.pdf]

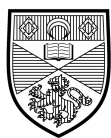

Editors  
Bayesian Analysis

4 July 2023

Dear Editors,

Submission number: **BA2205-011**

**Title: Bayesian inference for stochastic oscillatory systems using  
the phase-corrected Linear Noise Approximation**

Thank you very much for considering our paper for publication and inviting this for resubmission.

We have now responded to all the issues raised by the reviewer. Please find in supplementary files the point-by-point responses to the reviewer comments, and a marked version of the manuscript where the changes and the corresponding reviewer comment are noted clearly.

We thank you for your consideration and very much hope that you now find the paper ready for publication.

Yours sincerely,

Giorgos Minas

On behalf of the authors Ben Swallow, David A. Rand, and Giorgos Minas

# Responses to Review of BA-2205-011

Ben Swallow, David A. Rand, Giorgos Minas

July 4, 2023

*We thank the reviewer for their helpful comments, which has led to a much improved manuscript. Please find below the point-by-point responses to the reviewer's comments.*

**Overview** The submission considers data consisting of multiple replicates of noisy, cyclic stochastic systems. It uses the pcLNA, an algorithm proposed in an earlier article by two of the authors, as an approximation to the true model. This is first used to identify which parameters may be inferable from data. It is then used as the inference model. For the first data set, simulated via pcLNA, three different MCMC schemes are used, with parallel tempering mixing best and managing to identify a minor mode. The second data set (for a different system) is simulated from the true process, and only parallel tempering is used. When the system size is large, pcLNA does very well; decreasing the system size leads to some bias.

**Main thoughts** There are several ideas in this paper, and some potentially useful output, but it lacks a depth of comparison or crispness of the arguments and recommendations. Essentially there are three/four separate thrusts:

- pcLNA can be used for cyclic systems. It can be used to decide which parameters might be identifiable from the data via the FIM, and for inference on those parameters (with others fixed according to the literature).
- Inference via three different algorithms is tested on one example. The algorithms are a handicapped version of the RWMH, sMMALA and a parallel tempered RWMH (also handicapped). Only the final algorithm finds a minor mode. The presence of the minor mode is interesting - and being able to find it is, clearly, useful.
- the pcLNA posterior leads to values consistent with the true parameter values (at least for large systems). It is claimed that the simulation studies show that sensitivity analysis gives the identifiable parameters.

Some of these areas could and should be developed more, but there should also be some streamlining.

A. Use of the pcLNA FIM for sensitivity: currently, the parameters that might be identifiable are found and then inference is performed on these (with a few additional low-sensitivity parameters included when inference is on the log-scale). Except when some parts of the data are removed, the parameters with high sensitivity are well identified and those with low sensitivity are not. This could be much more systematic, with the choices mapped out more clearly for the reader. Sensitivity analysis is performed on the raw scale and on the log scale, and different patterns are found for each, leading to different sets of parameters that are, apparently, identifiable. What is the take home? What should the user do in their analysis, and why?

1. It seems to me that if a particular concentration is measured in mols/litre instead of mols/ml this would change the raw sensitivity of parameters associated with this particular  $x$  by a factor of 1000, but it's not "real". Furthermore, knowing a parameter is between 0.1 and 0.2 is very different to knowing it is between 10.1 and 10.2. These correspond to the same sensitivity on the raw scale. Each of these issues disappears if one uses the log scale. Is there a good reason to use the raw scale? If so, the pros and cons of the two possibilities should be discussed so the reader can decide which is most appropriate for them. If not, then the

log scale should be used and recommended throughout. This would make the description - and the message - much simpler. Indeed, if the reasons to use the raw scale are lesser in the examples in the paper then the sensitivity analyses could still be just on the log scale.

*Thanks for the suggestions. Regarding the raw- or log-scale question, we agree that in most cases the log-scale should be used for the reasons explained above. We included a discussion about this in the updated version. Regarding giving a more clear take-home message on this issue, we made several changes and additions. First we discussed the objectives of this study of the relation between sensitivity analysis and estimation and we clarified better the computations. We performed an analysis comparing MCMC runs outputs with the corresponding sensitivity coefficients. We now incorporated to the document a new section called "The relation of parameter estimates to the sensitivity coefficients" that discusses this issue.*

2. Please note that this is a completely separate question from whether inference (MCMC) should be performed on the log scale or not. It is the same posterior that you are exploring either way, it just might be more efficient to explore it on one or other scale. I suspect that if you precondition the RWMH sensibly from a tuning run (via the variance-covariance of either the raw parameters or the logged parameters) then both will mix reasonably.

*Yes that's correct. We noted that in the document.*

- B. From the figure, on the log scale, the parameters with largest sensitivity are TNFKB, ka, kd1a, kc2a, ki3a, c1a, c2a, c1, c2, c4 and dose. Yet TNFKB, dose and kbA20 were identified as highly sensitive, with kc1a and c5a deliberately included because they had low sensitivity. As a minor point, kbA20 does seem to be highly sensitive. More to the point, why were the other sensitive parameters not included - the choice seems to be arbitrary. The text says that all parameters were identifiable and it was only when some species were not observed that some parameters became not identifiable. There is much that could and should be teased apart here:

- 1 Is there a good reason for only choosing some of the sensitive parameters and only these specific ones? If so, give it! If not, try inference with all of them in. If this doesn't work (because the variances of some linear combinations are very large) then explain. The eigenvectors of the FIM matrix ought to tell you which parameters should be identifiable in combination. The reader needs some concrete take-homes.

The text says that parameters only because non-identifiable when observations were removed. Why were the parameters with low sensitivities identifiable when all the data was present?

*We included a much more thorough discussion on this matter, including estimating larger number of parameters, and estimating only low or only high sensitivity parameters. Please see answer to A1.*

- 2 It should be possible to find the FIM, when B is something other than the identity. So, include the sensitivities of the log parameters for this case too and use it to explain the findings for when you remove some of the observations.

*Yes this is possible. In fact we performed such analysis in Minas and Rand (2019). Since the matter of the use of sensitivity analysis for guiding estimation is more general, and the above will only answer a smaller question, we focused in thoroughly answering the general question in the updated document.*

- 3 In all cases it would be good to see some measure of how much more concentrated the posterior for each parameter is than the prior - this can then be compared directly with the predictions from the sensitivity analysis. Perhaps the KL divergence between the (marginal) prior and posterior? Or simply comparing the prior and posterior standard deviations? This would give greater confidence in the mechanism for choosing which parameters to fix and which to allow to vary, so that a reader might be able to apply the same ideas to their system. This would also better back up the claim in the discussion that "The sensitivity analysis was able to predict which parameters were estimable from observed data."

*Thanks for the suggestion. We added results comparing prior to posterior precision and showed how this compares to sensitivity coefficients. Please see the answer to A1.*

- C. Comparing MCMC algorithms: this is the weakest part. The RWMH algorithm is handicapped - preconditioning from an initial tuning run should be used. But more to the point, the main message is that there can be multiple modes, so parallel tempering is helpful. I would suggest straight away using parallel tempering (with pre-conditioning for the RWMH), and pointing out that other algorithms are possible, that two of these (RWMH - preconditioned - and sMMALA) were tried but that both failed to find the minor mode. Put the details of these two algorithms and the results in the appendix. (Aside: there was only a 35% improvement in effective sample size for sMMALA, but usually it is much slower than the random walk as it needs to calculate gradients and FIMs via the LNA - any comparison in the appendix should take computational time into account.) This also simplifies the message from the paper - you're saying to use parallel tempering. You can still perform parallel tempering on the log parameters or on the raw parameters. One of the really neat findings is the secondary mode in the first example - I explain later how the exploration of this aspect could be completed. This mode would still be present when the logs of the parameters are used. Just using the parameters  $c1a$  and  $c1$  is not really justified by the sensitivities on the log scale, but you could do this for illustrative purposes.

*We have added a comment that clarifies that the intention is not to compare the algorithms but to show the possibility of using them for these models, which is not documented in the literature, and to justify why all subsequent results are done using the PTMCMC algorithm.*

- D. Use of pcLNA: other inference techniques are available. For example, the restarting LNA of Fearnhead et al. using the KF or the SSA (or SDE) using particle MCMC. In at least one example we need to see a comparison of a state-of-the art technique and the pcLNA for inference (not for simulation - I understand that was done in the previous article). Is the inference much different (if using the restarting LNA do both posteriors fit with the true parameters; if using particle MCMC with the true data generating mechanism, how close is the pcLNA posterior to the true posterior)? What about computational time? On the comparison - the data in the first example are generated from the pcLNA - it would be better to use the SSA - else give a very good explanation as to why not.

*We compared the restarting LNA Kalman Filter in Fearnhead et al. with pcLNA in a new subsection. We coded the restarting LNA for computing the likelihood using code that is otherwise identical to the code used for pcLNA and discussed the results.*

- E. I found a large number of mistakes - mathematical mistakes, notational mistakes, non-words, as well as unclear explanations or missing information. This needs to improve dramatically in any revision.

*We went through the document in detail and tried to remove all mistakes. Thanks for pointing those out*

## Other detail

- F. Section 3 describes the LNA but does not even try to explain or give an intuition as to why this is a reasonable approximation to the system dynamics. In fact, even the SSA is never detailed. Yet some understanding of the true dynamics is needed to justify the pcLNA. This really needs a paragraph or two at the very least saying one of: (a) give the SSA, cite Kurz approximation; or (b) say that matching the first two moments of the changes to the populations in the true Markov model over time  $\Delta t$ , leads to the SDE approximation [full SDE], this is then approximated by expanding about the ODE solution and keeping only the lowest order terms that lead to tractability..."

*In the previous manuscript, our focus was on describing the model being used rather than how it is derived, but we see the benefits of describing the context in which it is derived. We now renamed the section "The pcLNA model" to "Reaction network dynamics and the pcLNA model" and included a description starting from the setting of reaction networks, developing the Poisson processes that describe them, and leading to the LNA that we think that enables the reader to understand the setting without getting into unnecessary details.*

- G. 1 Equation (3.6) is incorrect. There should be  $+SS^T$ , not  $+S$ . Please check that you did not use the incorrect expression in your runs.

*We changed the notation and made a correction to make this more clear. The code is correct. Thanks for the suggestion.*

- 2 p8 the factorisation of the likelihood is only correct if the observations are exact, as then the Markov property can be used. The observations are not exact (see (3.10)) so this factorisation is incorrect. The product should have terms  $P(\mathbf{y}_i|\mathbf{y}_0, \dots, \mathbf{y}_{i-1}; \boldsymbol{\theta})$ . The likelihood factor a few lines down also needs changing. Figure 2 also needs changing: the left most term is  $X_i|y_1, \dots, y_{i-1}$  and the output (beneath) is  $P(\mathbf{y}_i|\mathbf{y}_0, \dots, \mathbf{y}_{i-1})$ . Similarly, future terms need changing. These changes then need to follow through to the description of the algorithm - priors are  $(\mathbf{X}_i|\mathbf{y}_{0:i-1})$ , etc. The output of the algorithm also needs changing to  $P(\mathbf{y}_i|\mathbf{y}_{0:i-1})$

*All corrections made. Thanks for the reminder.*

- 3 p11 The only time one would run a RWMH with variance  $\sigma^2 I$ , would be as a very first initial run. After that one would always precondition - find an approximate posterior variance matrix, Cholesky decompose it (once) to  $LL^T$ , and use a proposal of  $\sigma LZ$ , where  $Z$  is a vector of  $N(0, 1)$  rvs. It is not reasonable to compare to the handicapped RWM algorithm presented - a preconditioned algorithm should be used. For the parallel tempering it would also be sensible to use a preconditioned RWM. It will mix so much faster.

*We had done significant pre-turning of the algorithms. Approaches formally using the covariance structure were actually found to be sub-optimal here given that there was dependence on which of the mode the chains were currently in. Arguably this is 'less' handicapped than the way that the other methods are run. Additional descriptions have been added to section 3.2.*

- 4 p13 I wonder if the acceptance probability for simulated tempering should be  $\min(1, e^{\Delta\beta\Delta E})$ . Please check this and that the correct probability was used in your algorithm. To see how to get the above expression, the acceptance ratio is  $\frac{\pi_j(\theta(j-1))\pi_{j-1}(\theta(j))}{\pi_j(\theta(j))\pi_{j-1}(\theta(j-1))}$ . The logarithm of this is  $\{l_j(\theta(j-1)) - l_j(\theta(j))\} - \{l_{j-1}(\theta(j-1)) - l_{j-1}(\theta(j))\}$  where  $l_j$  is the log posterior for chain  $j$ . But  $l_j = -\beta_j E$  so this expression is  $(\beta_j - \beta_{j-1})E[\theta(j)] - E[\theta(j-1)]$ .

*Yes you are correct and this is what was used in the code. A typo in the manuscript that has now been corrected.*

- 5 p15 The final paragraph in Section 4.1 is really important, and is in danger of being missed by a reader going straight to the MCMC results. At least a sentence on the fact that you use the sensitivity analysis to choose which parameters to fix at values from the literature and which to perform inference on should appear on p3. The para on p15 should also say exactly how many parameters you perform inference on in each case, and how many you fix.

*We now include a discussion explaining how we use the sensitivity analysis for estimation. Thanks for the suggestion.*

- 6 p15 Why aren't all trajectories simulated from the SSA? This should be the gold standard: simulate from the SSA - a good test of pcLNA is that it recovers (close to) the true parameters. (Aside: it's not stated which method was used for the first data set, the reader is left to work backwards when they later discover that the second system was simulated using the SSA.)

*The reason is that, although previous studies in Minas & Rand (2017) had shown strong agreement between pcLNA and the SSA, it is still sensible to first of all check the ability to retrieve the correct parameters from the assumed model (pcLNA) so that any discrepancies can be correctly allocated to either the likelihood approximation or the inference procedure.*

*We initially show we can retrieve the correct values where data are simulated from the pcLNA algorithm before then conducting further simulations such to show equivalence with the SSA too.*

- 7 p17 The existence of two modes is interesting and a success of the paper but a more complete explanation is needed. Figure 5 is part of the explanation but we really need the other part which is showing how the observations fit with both of the models. What you really need is a plot with all the data on it together with two filtering distributions (of whatever linear combination(s) of  $X$  are relevant to the data - via the  $B$  matrix): one at the true posterior

mode and one at the minor mode. Then the reader can see how the parameters settings correspond to very different paths and yet both can explain the data.

*We have modified this figure (Figure 9 in the new manuscript) to show the trajectories of the two modes and the data.*

- 8 p18 the formula with the Jacobian in isn't right as there is a single likelihood term for the whole vector  $\theta$ , whereas there are individual priors for each component of  $\theta$ , so the final term would be  $-P \log \theta_i$ .

*The formula presented in the manuscript was for a univariate  $\theta$  but we accept this is confusing when elsewhere  $\theta$  is a vector. In the algorithm we used, this was  $-\sum_i \log(\theta_i)$  as mentioned and we have altered the manuscript to reflect this.*

- 9 There's a further error, though. It is stated that the prior is specified on the original scale so shouldn't it be  $p(\exp(\theta))$  rather than  $p(\log \theta)$ . This could be explained much more clearly by setting  $\psi_i = \log \theta_i$  and then you have

$$\log \pi(\psi|\mathbf{y}) = \log f(\mathbf{y}|\psi) + X \log \pi(\exp(\psi_i)) - X\psi_i + \text{constant}$$

. (yes, the proportional sign in the submitted article is also incorrect).

*Corrected.*

- 10 You've overloaded  $\theta$  with two meanings, and the result has been confusion. If you end up doing everything on the log parameter scale, it would be simpler to just set the prior on this scale (e.g. a vague Gaussian) and then using a RWMH on this scale - then no Jacobian would be necessary.

*Thank you. This has all been updated to make it clearer. The reason we specify priors on the original scale is that it is often known roughly the order of magnitude of different parameters, and as many are rate parameters, gamma distributions are a natural choice. This can also alleviate some of the problems of non-identifiability in cases where deviation over some restricted parameter space may not have large impacts on inference (particular as our identifiability study is local not global). However, vague priors on the log scale are also a possible choice.*

Minor I noted the following points as I read the paper. Some may not fit with my thoughts after finishing reading the paper, as given above.

- H. 1 P1 Googling the word "doselitude" returns only three hits, including the article under review here. This suggests that most readers of statistics articles (including, but not limited to, this reviewer) will not understand it's meaning, nor be easily able to find out its meaning. Exactly the same three hits appear for the word "Exdoseles". The article should explain these words as they are used - or use some other, more commonly seen words.

*Changed "doselitude" to "amplitude", "Exdoseles" to "Examples". This was a find and replace of "amp" (name of dose parameter in software) to "dose" seriously backfiring. Please accept our sincere apologies for this.*

- 2 P2 "Traditionally oscillations are modelled. . . ." My understanding is that its the stochasticity in the period that renders the deterministic models next to useless. If there were just stochasticity in the exact path taken over each periodic cycle, this wouldn't be such an issue. It would be worth making this point clear in this paragraph.

*We made changes in this and the next paragraph to highlight this point and that the pcLNA method overcomes the problem. Note that we discuss this in more detail in p.7 paragraph starting with "The accuracy of the standard LNA . . .".*

- 3 P2 "Therefore the use of approximate simulation methods, such as Approximate Bayesian Computation" - for the type of data that have been described and for which the pcLNA would be appropriate, particle MCMC would be more efficient since it includes the observation likelihood conditional on the stochastic process and there is no need for summary statistics and approximation. I would mention that in preference to ABC.

*Thanks for the suggestion. We added a comment for this and a reference.*

- 4 P3 “this making exact parameter estimation methods” - this is not strictly incorrect, but it is misleading. MCMC performs exact inference but it would be on an approximate model. Can this be clarified?  
*Agree. We changed “exact” to “likelihood-based”.*
- 5 P4 “has been shown to be highly stochastic Tay et al. (2010b)” should be “. . . (Tay et al., 2010b)”  
*Done. Thanks.*
- 6 p4 the 11-dimensional system you use is a reduced version of the model of Ashall et al.. The para then says that the model of Ashall et al. has 31 parameters. But what we really care about is how many parameters are in the reduced version which you’re using.  
*Done. We clarify that the model used has 31 parameters.*
- 7 p4 “Estimation .. extremely important . . . ” please can you remove the hyperbole? Indeed, this whole sentence could be removed.  
*DONE. Thanks.*
- 8 p5 Figure 1 is not referred to from the text - any figure worth including should be discussed in the text. Moreover, it would motivate the pcLNA methodology much better if you showed SSA simulations of the systems. Then in the left figure we could see the differing periods.  
*We added the SSA simulated data for the clock system here.*
- 9 p5 “about an unknown parameter  $\theta$ ” -  $\theta$  should be bold.  
*Done. Thanks.*
- 10 p6 “there is an  $s \times s$  orthogonal matrix” - do you mean orthonormal matrix? With an orthogonal matrix you could make all the  $\sigma_i = 1$ . With an orthonormal matrix they must be the eigenvalues of the FIM as stated a few lines further on.  
*The matrix is orthonormal. The term orthogonal matrix is commonly used as equivalent to orthonormal matrix. This part is slightly changed to become more clear. See H12.*
- 11 p6 “the matrix V diagonalises it” - no such matrix has been defined. You mean bold A.  
*DONE. Changed to **A**. Thanks.*
- 12 p6 Why talk about SVD? For a square, symmetric matrix it is much cleaner to talk about the spectral decomposition, which is what you have. The SVD generalises this to non-square matrices. Moreover, you are now using V (not bold) where you used A (bold) before. Please be consistent, both in symbol choice and whether or not matrices are bold. Finally V is orthonormal, not just orthogonal.  
*DONE. We changed this part slightly to make it more clear.*
- 13 p6 (3.2) defines F - please say this.  
*DONE. Thanks.*
- 14 p6 (last para) (1) “state change after the occurrence of the j-th transition” you mean “j-th reaction type” or “j-th type of transition” - the jth transition is simply that - and could be any one of the possible transitions. (2) “transition that occurs with rate”. Clearer English would be “transition; a transition that occurs with rate” - except “transition” should be replaced with “transition type” or “reaction type”.  
*DONE. We clarified this paragraph. Thanks for the suggestions.*
- 15 p7 top bullet: the equation for  $S^2$  is only correct if S is square and symmetric. It should be that S is any matrix with  $SS^T = ARA^T$ . Btw, again, please be consistent - are matrices all bold or all lower case? What dimension is the Wiener process? You can get away with R, but if you set  $S = A$  it is N-dimensional.  
*DONE. The matrix **S** is square and symmetric because it is the (unique) square root of the (positive definite) matrix  $\mathbf{A}\mathbf{R}(\varphi(t))\mathbf{A}^T$ . Hence the equation is correct. We are aware that the matrix **S** is more commonly defined as  $\mathbf{S} = (\mathbf{A}\mathbf{R}(\varphi(t))\mathbf{A}^T)^{1/2}$ , but we prefer the more compact definition used here.*  
*It’s not clear here but we suspect the inconsistencies is suggested because, in the first manuscript, we used bold upper case letters for random vectors as well as matrices. In*



the updated manuscript, we use bold lower case for all vectors and bold upper case for all matrices. When the vectors are random we make this clear in the text. We hope this notation is more clear. We created a footnote stating this notation.  
The Wiener process is  $N$ -dimensional. We noted this in the updated version. Thanks for pointing this out.

- 16 p7 “Equation (3.4) implies that if  $\xi_{t_0}$  is  $MVN \dots P(X(t_1)|X(t_0))$  is  $MVN$ .” This is not quite right. In your conditional probability you are conditioning on the value at  $t_0$ , so it doesn’t matter what distribution it came from as it is treated as a constant! If it came from a  $MVN$  then the marginal distribution  $P(X(t_1))$  is  $MVN$ . Indeed, if it came from a  $MVN$  then the joint distribution at any sequence of times is also  $MVN$  as you say in the next line. The word “tridiagonal” should be replaced with “block tridiagonal”. The precision matrix is not tridiagonal as there can be any type of dependence between the  $N$  populations - it’s just tridiagonal across time points.

*DONE. The reviewer’s comment about the conditional distribution  $\mathbf{x}(t)$  given a constant value of  $\mathbf{x}(t_0)$ ,*

$$P(\mathbf{x}(t)|\mathbf{x}(t_0) = \mathbf{x}_0)$$

*is correct, but the sentence refers to the more general case of the conditional distribution of  $\mathbf{x}(t)$  given that  $\xi(t_0)$  and in turn  $\mathbf{x}(t_0)$  is  $MVN$ . This more general case ensures that the joint probability distribution of  $(\mathbf{x}(t_0), \mathbf{x}(t_1), \dots, \mathbf{x}(t_n))$  is also  $MVN$ . We clarified this in the updated version.*

*The reviewer’s comment about the tridiagonal form is correct. That’s what we meant to write, and we now used the term “block tridiagonal” as suggested. Thanks.*

- 17 p8 prior to this page,  $t_0$  was an initial condition (though I couldn’t find this stated). For pcLNA the top paragraph describes frequently correcting the phase, and now  $t_0$  is any time at which a phase correction is used. It would be helpful to make clear for the LNA and then the pcLNA what exactly  $t_0$  is.

*DONE. We clarified this in the updated manuscript. In fact, we updated the description of pcLNA to become more clear, added a diagram, and gave insights for the underlying idea. As part of this, we moved the pcLNA equations from the Kalman Filter section to the section describing pcLNA.*

- 18 p8 (3.10) bold  $\epsilon$  has not been defined at all, and certainly not to be the concatenation of all the vectors bold  $\epsilon_i$ , similarly bold  $X$ . So (3.10) should end with a text line saying all bold  $\epsilon_i$  are independent of each other and of all bold  $X_j$ .

*DONE. This is now clarified.*

- 19 p9 I cannot find where the term  $y - 1$  in Fig 2 is defined. Indeed, Step KF1 in the algorithm says the first observation is  $y_0$ .

*DONE.  $\mathbf{y}_{-1}$  denotes the prior mean and variance. We clarified this better in the updated manuscript.*

- 20 p10 Comparing Step KF3b with (3.8) and (3.12) suggests that  $X$  is its posterior expectation. Why? Can you add a pointer from this step to where it explains this in the text?

*DONE. That’s not correct. It’s not entirely clear why this confusion arises exactly and instead of guessing, we would be pleased if more explanation is given. The notation is slightly changed there, and hopefully that helps avoid this confusion.*

- 21 p10 In the algorithm description the phase is only updated at observation times; whereas earlier in the text it has been stated that the phase needed to be updated several times per cycle. The text should explain the apparent discrepancy here.

*We added a paragraph to explain this.*

- 22 p11 (top) In addition to the use of phase shifts, the other major difference between this algorithm and the restarting LNA of Fearnhead et al. is that the pcLNA algorithm does not restart the numerical integration. The fundamental issue is deviations from the ODE path as when these become large the LNA becomes inaccurate. Fearnhead et al. deals with this by restarting the ODE integration. The pcLNA deals with it by finding the closes point in the ODE path to the current and shifting to that point. The latter is computationally



quicker as it does not need to reintegrate, but it does rely on there being a point on the ODE path that is close enough to  $X$  (or its posterior mean) for the path point to be representative. I think these points, and the contrast, could and should be made more clearly.

*We discussed this issue in the section comparing pc- and restarting-LNA. The pcLNA assumes that the system has a limit cycle solutions and performs oscillations around this. If the time-series stop oscillating (e.g. drift away of the limit cycle), then the pcLNA fit will be poor and another method needs to be used. We made clear throughout the assumptions on the system dynamics and more details included in Minas and Rand (2017).*

- 23 p11/12 What is a Gibbs sdoeseler? and sdosele size? past sdoseles? and many more - It's almost as if you've done a search and replace on "amp" to "dose".

*Done. That's exactly what happened. Apologies.*

- 24 p13 In Step 1, the  $\theta$  and  $\theta^*$  must be indexed by  $j$  (e.g.  $\theta^*(j)$  - as you're doing this for each of the  $j$  chains separately - you're not proposing a single  $\theta^*$  for all chains.

*DONE.*

- 25 p13 Similarly, the energy function is the same for each chain so should not be indexed by  $j$  - it's just the  $\theta$  that is applied to which differs, so  $E[\theta]$  should be  $E[\theta(j)]$  (there is a typo in that  $t - 1$  should not be used at all.  $jt - 1t$

*DONE.*

- 26 p13 There's a similar indexing problem and lack of clarity with Step 2. It would be clearer to say: For the  $j$ -th and  $(j - 1)$ -th chains, accept a swap of:  $\theta(j) \leftrightarrow \theta(j - 1)$  with a probability of [see earlier point]. Also,  $\Delta E$  should be more clearly defined as  $E[\theta(j)] - E[\theta(j - 1)]$ .

*DONE.*

- 27 p13 "with other chains . . . subsequently discarded" - this is a waste - the other samples can be given importance weights and used within any posterior averaging. At the very least you could point out that any efficiency this method achieves by discarding the other samples is a lower bound on the actual efficiency that would be obtained by reusing all samples..

*DONE. Yes, we could use an importance smapling approach to combine the resulting chains, however this is beyond the scope of the paper. We have added a statement to this effect.*

- 28 p13 "with parameter changes in the log scale" - I initially mis-understood this as you having logged the parameters and found the FIM wrt the logged parameters,  $\psi_i = \log \theta_i$  and the eigenvalues of this matrix. Or maybe this is what you did? Can this sentence be made clearer? Similarly in the caption to the figure. If this is what you did, why not also do it for Drosophila? Given the better behaviour on the logged scale it might make sense to use the logged parameters for the RWMH and other algorithms rather than the raw parameters (this would also stop you proposing negative values for any of the parameters). Later on in the paper, it says that you do this. So perhaps you could make the link here too?

*We used the log-scale for drosophila and this should be clear in the updated documents. We also made more clear when we plot eigenvalues and/or sensitivity coefficients in the log-scale.*

- 29 p14 Fig 3(b) seems to be much more useful than Fig 3(a). The absolute scale simply depends on the amount of data. So Fig 3(a) is simply saying that there comparatively less information for Drosophila.

*We feel they both provide useful information and we wish to keep them in.*

- 30 p14 "in log case, base 2" - I do not know what this means. All three of (c)-(e) are on the log scale, presumably. Do you mean that when the logarithms of the parameters are taken, the log is base 2? If so, it would be clearer to say it when describing (c)?

*There is a typo here: "case" should be "scale", which is now corrected. This sentence talks about sensitivity coefficients and says that in the heatmaps the sensitivity coefficients are in log scale, with base 2. The parameters are either in raw or log scale and this is stated in the description of c,d and e. As it refers to all plots c-e, we think the note is placed correctly. We made some changes in the colouring of the figure to reduce visibility issues related to colour-blindness. We also made the wording in the caption more clear.*

- 31 p14 Fig 3(b). It would be useful to have the equivalent of this plot but including all of the eigenvalues, not just the first 10 - perhaps in the appendix, but referred to from the main text. Then we would have a clear idea of exactly what fraction of the eigenvectors would be difficult to estimate.

*We have added these plots in the Appendix.*

- 32 p14 The caption to figure 3 contains commentary: “The NF-kB system overall has larger sensitivities, but the FIM is dominated by few eigen-directions, while the clock model is more balanced in parameter sensitivities.” and “Fewer parameters . . . clock.” This should be in the main text, not the caption.

*We would like the main message of some key figures to be given briefly in the caption.*

- 33 H33 - p15. The model for the data (3.10) has Gaussian noise in it. What noise was added? What B matrix was used? How many observations were taken each cycle? How many cycles was the system followed for? How many independent replicates? This information is important for anyone wishing to replicate your experiments. The bottom of p18 says that B is no longer the identity, but I couldn’t see where it was said that, originally, it was the identity.

*We clarified this in the updated document.*

- 34 p19 “the dose parameter reverted to the prior mean of approximately 10” - this means that the posterior for the dose parameter was close to a delta function at 10 - not what you intended. Hopefully, what you wanted to say was that the marginal posterior distribution was close to the prior distribution, with approximately the same mean and variance. What you might be trying to say is that the posterior and prior means were the same - but that doesn’t fit with the “no information” that the rest of the paragraph is saying - the posterior could be much tighter about 10 than the prior.

*We did mean that the posterior distribution becomes almost identical to the prior distribution in this case and the text has been updated to clarify this. Also an additional plot has been added (Figure 10) to visualise this.*
